# Supplementary material for: Sequential infection experiments for quantifying innate and adaptive immunity during influenza infection
Source: arXiv:1709.02145 ancillary file (2018-06-05)
Supplement: Supplementary file 1 [file S1_File.pdf]

# Sequential infection experiments for quantifying innate and adaptive immunity during influenza infection

S1 File:

Two-strain model equations for the baseline and modified models,  
and compartmental diagrams for the modified models



# 1 The two-strain baseline model

The model equations are given by

$$\frac{dT}{dt} = g(T + R) \left( 1 - \frac{T + R + \sum_{q=1}^2 I_q}{T_0} \right) - \sum_{q=1}^2 \beta V_{inf,q} T + \rho R - \phi F T, \quad (1a)$$

$$\frac{dI_q}{dt} = \beta V_{inf,q} T - \left( \delta_I + \kappa_F F + \sum_{j=1}^J \kappa_{Ejq} E_j \right) I_q, \quad q = 1, 2, \quad (1b)$$

$$\frac{dV_{inf,q}}{dt} = \frac{pV_{inf}}{1 + sF} I_q - (\delta_{V_{inf}} + \kappa_A A_q + \beta T) V_{inf,q}, \quad (1c)$$

$$\frac{dV_{tot,q}}{dt} = \frac{pV_{inf} pV_{ratio} \alpha}{1 + sF} I_q - \delta_{V_{tot}} V_{tot,q} - \alpha \beta T V_{inf,q}, \quad (1d)$$

$$\frac{dR}{dt} = \phi F T - \rho R, \quad (1e)$$

$$\frac{dF}{dt} = \sum_{q=1}^2 I_q - \delta_F F, \quad (1f)$$

$$\frac{dB_{0q}}{dt} = - \frac{V_{tot,q}}{k_B + V_{tot,q}} \beta_B B_{0q}, \quad (1g)$$

$$\frac{dB_{1q}}{dt} = \frac{V_{tot,q}}{k_B + V_{tot,q}} \beta_B B_{0q} - \left( \frac{n_B}{\tau_B} + \delta_B \right) B_{1q}, \quad (1h)$$

$$\frac{dB_{iq}}{dt} = \frac{2n_B B_{i-1,q}}{\tau_B} - \left( \frac{n_B}{\tau_B} + \delta_B \right) B_{iq}, \quad i = 2, \dots, n_B, \quad (1i)$$

$$\frac{dP_q}{dt} = \frac{2n_B B_{n_B,q}}{\tau_B} - \delta_B P_q, \quad (1j)$$

$$\frac{dA_q}{dt} = P_q - \delta_A A_q, \quad (1k)$$

$$\frac{dC_j}{dt} = \frac{M_j}{\tau_M} - \frac{\sum_{q=1}^2 I_q / k_{Cjq}}{1 + \sum_{q=1}^2 I_q / k_{Cjq}} \beta_C C_j, \quad (1l)$$

$$\frac{dE_{1j}}{dt} = \frac{\sum_{q=1}^2 I_q / k_{Cjq}}{1 + \sum_{q=1}^2 I_q / k_{Cjq}} \beta_C C_j - \left( \frac{n_E}{\tau_E} + \delta_E \right) E_{1j}, \quad (1m)$$

$$\frac{dE_{ij}}{dt} = \frac{2n_E E_{i-1,j}}{\tau_E} - \left( \frac{n_E}{\tau_E} + \delta_E \right) E_{ij}, \quad i = 2, \dots, n_E - 1, \quad (1n)$$

$$\frac{dE_{n_E}}{dt} = \frac{2n_E E_{n_E-1,j}}{\tau_E} - \delta_E E_{n_E}, \quad (1o)$$

$$E_j = \sum_{i=1}^{n_E} E_{ij}, \quad (1p)$$

$$\frac{dM_j}{dt} = \epsilon \delta_E E_{n_E} - \delta_E M_j - \frac{M_j}{\tau_M}. \quad (1q)$$

For the baseline model, the number of T cell pools is  $J = 3$ .

## 2 Models XC, XI and XIT

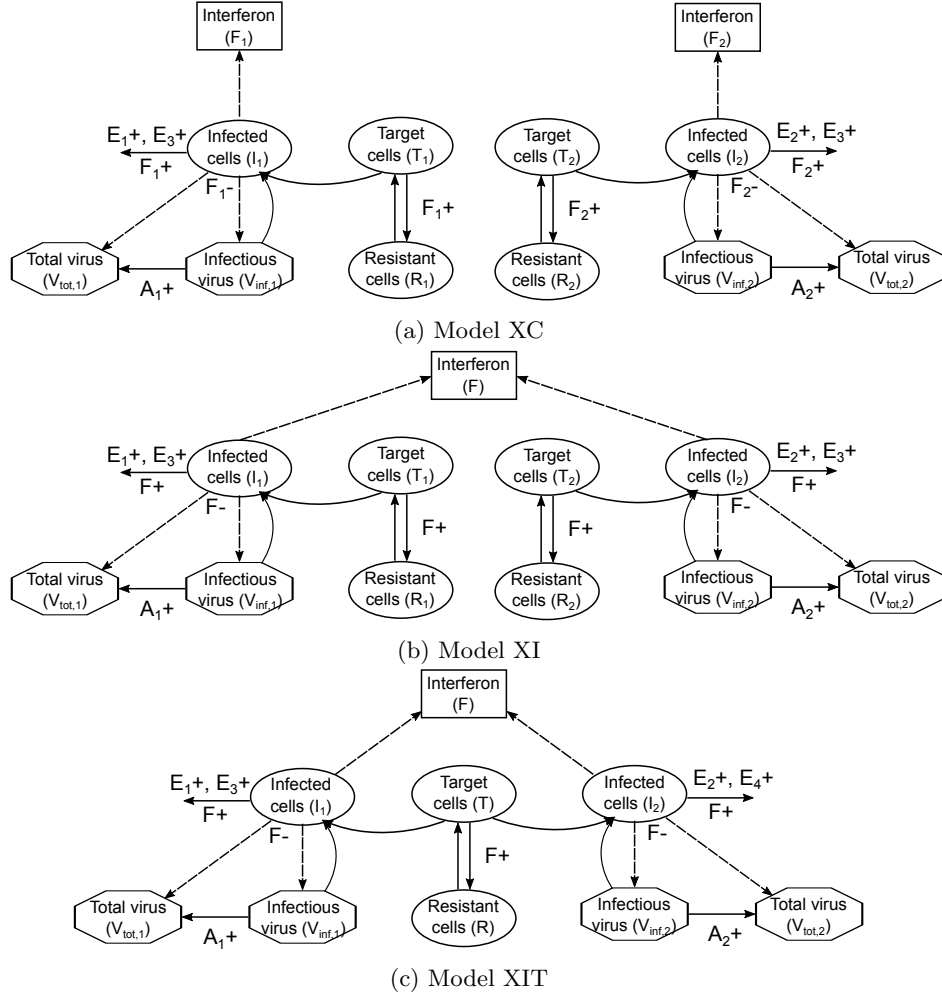

Figure 1: **Compartmental diagrams for models XC, XI and XIT.**

Figure 1 shows compartmental diagrams for models XC, XI and XIT. In model XC, cross-protection is mediated by cellular adaptive immunity only, and not target cell depletion or innate immunity. Unlike the baseline model, type I interferon  $F_q$  are strain-specific. Cells infected with strain  $q$  induce the production of interferon specific to that strain. The effects of interferon  $F_q$  —

rendering target cells temporarily resistant to infection; lowering the production rate of virions; and increasing the death rate of cells — only apply to strain  $q$ . In addition, each strain now targets a separate pool of uninfected cells; the size of each target cell pool is  $T_0$  (identical for both strains). This alternative model is not meant to reflect a biologically realistic situation; however, it enables *in silico* thought experiments to determine, for a given set of parameters, the contribution of each immune component to cross-protection.

Explicitly, the changed equations (relative to Eq. 1) for model XC are given by

$$\frac{dT_q}{dt} = g(T_q + R_q) \left( 1 - \frac{T_q + R_q + I_q}{T_0} \right) - \beta T_q V_{inf,q} - \phi F_q T_q + \rho R_q, \quad q = 1, 2, \quad (2a)$$

$$\frac{dI_q}{dt} = \beta V_{inf,q} T_q - \left( \delta_I + \kappa_F F_q + \sum_{j=1}^J \kappa_{Ejq} E_j \right) I_q, \quad (2b)$$

$$\frac{dV_{inf,q}}{dt} = \frac{pV_{inf}}{1 + sF_q} I_q - [\delta_{Vinf} + \kappa_A A_q + \beta T_q] V_{inf,q}, \quad (2c)$$

$$\frac{dV_{tot,q}}{dt} = \frac{pV_{inf} pV_{ratio} \alpha}{1 + sF_q} I_q - \delta_{Vtot} V_{tot,q} - \alpha \beta T_q V_{inf,q}, \quad (2d)$$

$$\frac{dR_q}{dt} = \phi F_q T_q - \rho R_q, \quad (2e)$$

$$\frac{dF_q}{dt} = I_q - \delta_F F_q. \quad (2f)$$

The equations for  $B_{iq}$ ,  $P_q$ ,  $A_q$ ,  $C_j$ ,  $E_{ij}$  and  $M_j$  remain unchanged.

In model XI, cross-protection is mediated by innate immunity, but not target cell depletion or cellular adaptive immunity. The model is altered from the baseline model such that the number of T cell pools is  $J = 4$ . T cell pools 3 and 4 have the same parameters as pool 3 in the baseline model, but T cell pool 3 is stimulated by, and targets, cells infected with strain 1 only, while T cell pool 4 is stimulated by, and targets, cells infected with strain 2 only. (Explicitly, the cross-reactivity parameters for T cell pools 3 and 4 are  $k_{C31} = k_{C42}$  equal to  $k_{C31} = k_{C32}$  in the baseline model;  $k_{C32} = k_{C41} = \infty$ ;  $\kappa_{E31} = \kappa_{E42}$  equal to  $\kappa_{E31} = \kappa_{E32}$  in the baseline model; and  $\kappa_{E32} = \kappa_{E42} = 0$ .) The cross-reactivity parameters for pools 1 and 2 remain the same. In addition, each strain now has its own target cell pool.

The equations for model XI which are altered relative to Eq. 1 are

$$\frac{dT_q}{dt} = g(T_q + R_q) \left( 1 - \frac{T_q + R_q + I_q}{T_0} \right) - \beta T_q V_{inf,q} - \phi F T_q + \rho R_q, \quad q = 1, 2, \quad (3a)$$

$$\frac{dI_q}{dt} = \beta V_{inf,q} T_q - \left( \delta_I + \kappa_F F + \sum_{j=1}^J \kappa_{Ejq} E_j \right) I_q, \quad (3b)$$

$$\frac{dV_{inf,q}}{dt} = \frac{pV_{inf}}{1 + sF} I_q - [\delta_{V_{inf}} + \kappa_A A_q + \beta T_q] V_{inf,q}, \quad (3c)$$

$$\frac{dV_{tot,q}}{dt} = \frac{pV_{inf} pV_{ratio} \alpha}{(1 + sF)} I_q - \delta_{V_{tot}} V_{tot,q} - \alpha \beta T_q V_{tot,q}, \quad (3d)$$

$$\frac{dR_q}{dt} = \phi F T_q - \rho R_q. \quad (3e)$$

In the model where cross-protection is mediated by target cell depletion and/or innate immunity, but not cellular adaptive immunity (model XIT), the cellular adaptive immune response is no longer cross-reactive. Like for model XI, the model is altered from the baseline model such that the number of T cell pools is  $J = 4$ . However, like the baseline model, target cells are shared between the two strains. Hence, the alterations in Eq. 3 are not made for model XIT.

### 3 Models where only one innate immune mechanism mediates cross-protection

We define the models XI1–XI3 (Fig. 2) such that in each model, cells infected with strain  $q$  induce the production of interferon specific to strain  $q$ . In model XI $y$ , cross-protection is only mediated by innate immune mechanism  $y$ , and not by the other innate immune mechanisms, target cell depletion, or cellular adaptive immunity. To recap, the three mechanisms are:

1. rendering target cells temporarily resistant to infection ( $T \rightarrow R$ );
2. decreasing the production rate of virions from infected cells; and
3. increasing the decay rate of infected cells.

Equations 4–6 show the equations which are changed in models XI1–XI3 relative to the baseline model (Eq. 1).

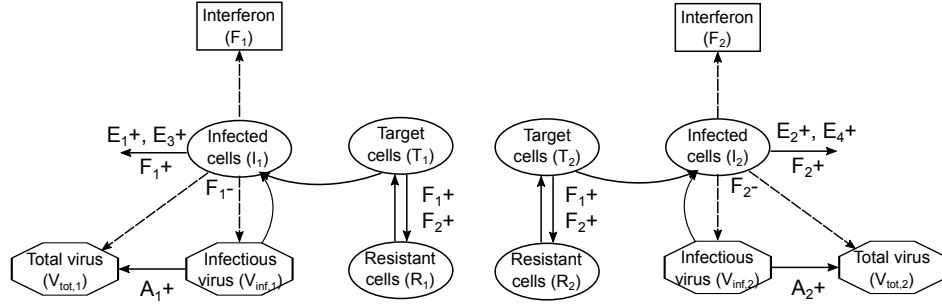

(a) Model XI1: cross-protection mediated by interferon rendering target cells temporarily resistant to infection

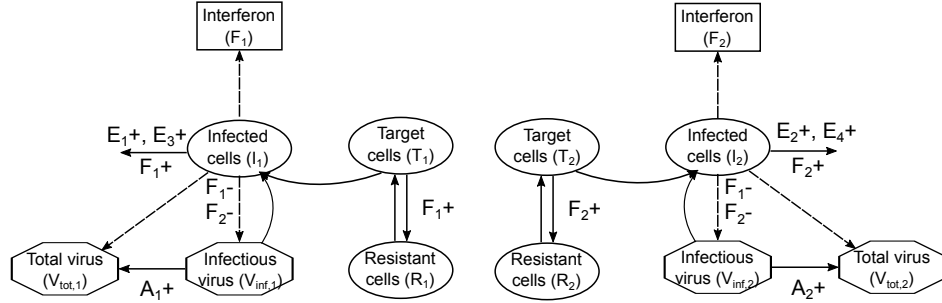

(b) Model XI2: cross-protection mediated by interferon decreasing the production rate of virions from infected cells

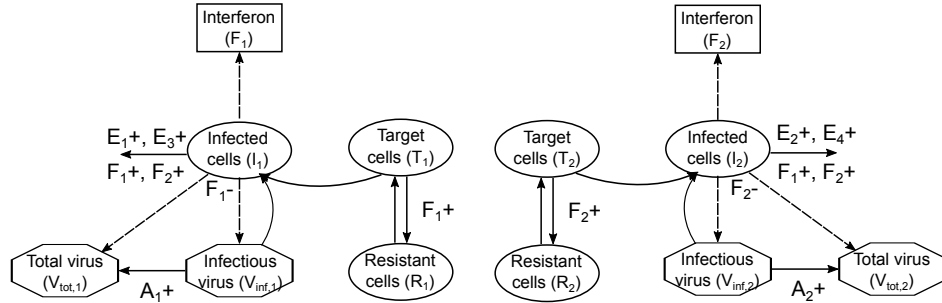

(c) Model XI3: cross-protection mediated by interferon increasing the clearance rate of infected cells

Figure 2: Three alternative models, where in model XI $y$ , cross-protection is only mediated by innate immune mechanism  $y$ , and not by the other innate immune mechanisms, target cell depletion, or cellular adaptive immunity.

$$\frac{dT_q}{dt} = g(T_q + R_q) \left( 1 - \frac{T_q + R_q + I_q}{T_0} \right) - \beta T_q V_{inf,q} - \phi \left( \sum_{q'=1}^2 F_{q'} \right) T_q + \rho R_q, \quad (4a)$$

$$\frac{dI_q}{dt} = \beta V_{inf,q} T_q - \left( \delta_I + \kappa_F F_q + \sum_{j=1}^J \kappa_{Ejq} E_j \right) I_q, \quad (4b)$$

$$\frac{dV_{inf,q}}{dt} = \frac{pV_{inf}}{1 + sF_q} I_q - [\delta_{Vinf} + \kappa_A A_q + \beta T_q] V_{inf,q}, \quad (4c)$$

$$\frac{dV_{tot,q}}{dt} = \frac{pV_{inf}pV_{ratio}\alpha}{1 + sF_q} I_q - \delta_{Vtot} V_{tot,q} - \alpha \beta T_q V_{inf,q}, \quad q = 1, 2, \quad (4d)$$

$$\frac{dR_q}{dt} = \phi \left( \sum_{q'=1}^2 F_{q'} \right) T_q - \rho R_q, \quad (4e)$$

$$\frac{dF_q}{dt} = I_q - \delta_F F_q. \quad (4f)$$

$$\frac{dT_q}{dt} = g(T_q + R_q) \left( 1 - \frac{T_q + R_q + I_q}{T_0} \right) - \beta T_q V_{inf,q} - \phi F_q T_q + \rho R_q, \quad (5a)$$

$$\frac{dI_q}{dt} = \beta V_{inf,q} T_q - \left( \delta_I + \kappa_F F_q + \sum_{j=1}^J \kappa_{Ejq} E_j \right) I_q, \quad (5b)$$

$$\frac{dV_{inf,q}}{dt} = \frac{pV_{inf}}{1 + s \left( \sum_{q'=1}^2 F_{q'} \right)} I_q - [\delta_{Vinf} + \kappa_A A_q + \beta T_q] V_{inf,q}, \quad (5c)$$

$$\frac{dV_{tot,q}}{dt} = \frac{pV_{inf}pV_{ratio}\alpha}{1 + s \left( \sum_{q'=1}^2 F_{q'} \right)} I_q - \delta_{Vtot} V_{tot,q} - \alpha \beta T_q V_{inf,q}, \quad q = 1, 2, \quad (5d)$$

$$\frac{dR_q}{dt} = \phi F_q T_q - \rho R_q, \quad (5e)$$

$$\frac{dF_q}{dt} = I_q - \delta_F F_q. \quad (5f)$$



$$\frac{dT_q}{dt} = g(T_q + R_q) \left( 1 - \frac{T_q + R_q + I_q}{T_0} \right) - \beta T_q V_q - \phi F_q T_q + \rho R_q, \quad (6a)$$

$$\frac{dI_q}{dt} = \beta V_q T_q - \left[ \delta_I + \kappa_F \left( \sum_{q'=1}^2 F_{q'} \right) + \sum_{j=1}^J \kappa_{Ejq} E_j \right] I_q, \quad (6b)$$

$$\frac{dV_{inf,q}}{dt} = \frac{p_{Vinf}}{1 + sF_q} I_q - [\delta_{Vinf} + \kappa_A A_q + \beta T_q] V_{inf,q}, \quad (6c)$$

$$\frac{dV_{tot,q}}{dt} = \frac{p_{Vinf} p_{Vratio} \alpha}{1 + sF_q} I_q - \delta_{Vtot} V_{tot,q} - \alpha \beta T_q V_{inf,q}, \quad q = 1, 2, \quad (6d)$$

$$\frac{dR_q}{dt} = \phi F_q T_q - \rho R_q, \quad (6e)$$

$$\frac{dF_q}{dt} = I_q - \delta_F F_q. \quad (6f)$$
