# Supplementary material for: Sequential infection experiments for quantifying innate and adaptive immunity during influenza infection
Source: arXiv:1709.02145 ancillary file (2018-06-05)
Supplement: Supplementary file 3 [file S1_table.pdf]

# S1 Table

| Parameter                                  | Description                                                                    | Value                         | Prior bounds                | Units                                                |
|--------------------------------------------|--------------------------------------------------------------------------------|-------------------------------|-----------------------------|------------------------------------------------------|
| $\log_{10} R_0$                            | basic reproduction number                                                      | $\log_{10} 4.9$               | [0, 3] [4, 7, 9, 12, 13, 1] |                                                      |
| $\log_{10} r$                              | initial viral growth rate                                                      | $\log_{10} 6.56$              | [0, 2] [4, 7, 9, 12, 13, 1] | day <sup>-1</sup>                                    |
| $\log_{10} \delta_I$                       | infected cell decay rate                                                       | $\log_{10} 2$                 | [-1, 2] [10]                | day <sup>-1</sup>                                    |
| $\log_{10}(\delta_{Vinf} - \delta_{Vtot})$ | difference between infectious and total virion decay rates                     | $\log_{10} 2$                 | [-2, 2] [11]                | day <sup>-1</sup>                                    |
| $\log_{10} \delta_{Vtot}$                  | total virion decay rate                                                        | $\log_{10} 8$                 | [0, 2] [10]                 | day <sup>-1</sup>                                    |
| $\log_{10} T_0$                            | initial number of target cells                                                 | $\log_{10}(7 \times 10^7)$    | [7, 8] [11]                 | target cell                                          |
| $\log_{10} g$                              | target cell regrowth rate                                                      | $\log_{10} 0.8$               | [-10, 0.5] [8, 5, 6, 3, 2]  | day <sup>-1</sup>                                    |
| $\log_{10} pVratio$                        | ratio of production of total to infectious virions                             | $\log_{10}(4 \times 10^4)$    | [0, 6]                      |                                                      |
| $\log_{10} \alpha$                         | the number of RNA copies/100 $\mu$ L of nasal wash corresponding to one virion | $\log_{10} 0.01$              | [-3, -1]                    | RNA copies/100 $\mu$ L virion <sup>-1</sup>          |
| $\log_{10} \gamma$                         | the initial ratio of total to infectious virions                               | $\log_{10}(4 \times 10^4)$    | [0, 5]                      |                                                      |
| $\log_{10} V_{inf0}$                       | the number of infectious virions upon exposure                                 | $\log_{10} 1$                 | [0, 3]                      | virion                                               |
| $\log_{10} \beta$                          | infectivity parameter                                                          | $\log_{10}(5 \times 10^{-7})$ | [-12, -4] [10]              | virion <sup>-1</sup> day <sup>-1</sup>               |
| $\log_{10} pVinf$                          | production rate of infectious virions by infected cells                        | $\log_{10} 12.6$              | [-6, 6] [10]                | virion infected cell <sup>-1</sup> day <sup>-1</sup> |

## References

- [1] Handel A, Longini Jr IM, Antia R. Neuraminidase inhibitor resistance in influenza: assessing the danger of its generation and spread. *PLoS Comput Biol.* 2007;3(12):e240. doi:10.1371/journal.pcbi.0030240.
- [2] Miao H, Hollenbaugh JA, Zand MS, Holden-Wiltse J, Mosmann TR, Perelson AS, et al. Quantifying the early immune response and adaptive immune response kinetics in mice infected with influenza A virus. *J Virol.* 2010;84(13):6687–6698. doi:10.1128/JVI.00266-10.
- [3] Pawelek KA, Huynh GT, Quinlivan M, Cullinane A, Rong L, Perelson AS. Modeling within-host dynamics of influenza virus infection including immune responses. *PLoS Comput Biol.* 2012;8(6):e1002588. doi:10.1371/journal.pcbi.1002588.
- [4] Saenz RA, Quinlivan M, Elton D, MacRae S, Blunden AS, Mumford JA, et al. Dynamics of influenza virus infection and pathology. *J Virol.* 2010;84(8):3974–3983. doi:10.1128/JVI.02078-09.
- [5] Smith AM, Perelson AS. Influenza A virus infection kinetics: quantitative data and models. *Wiley Interdiscip Rev Syst Biol Med.* 2011;3(4):429–445. doi:10.1002/wsbm.129.
- [6] Baccam P, Beauchemin C, Macken CA, Hayden FG, Perelson AS. Kinetics of influenza A virus infection in humans. *J Virol.* 2006;80(15):7590–7599. doi:10.1128/JVI.01623-05.
- [7] Petrie SM, Butler J, Barr IG, McVernon J, Hurt AC, McCaw JM. Quantifying relative within-host replication fitness in influenza virus competition experiments. *J Theor Biol.* 2015;382:259–271. doi:10.1016/j.jtbi.2015.07.003.
- [8] Petrie SM, Guarnaccia T, Laurie KL, Hurt AC, McVernon J, McCaw JM. Reducing uncertainty in within-host parameter estimates of influenza infection by measuring both infectious and total viral load. *PLoS ONE.* 2013;8(5):e64098. doi:10.1371/journal.pone.0064098.
- [9] Möhler L, Flockerzi D, Sann H, Reichl U. Mathematical model of influenza A virus production in large-scale microcarrier culture. *Biotechnol Bioeng.* 2005;90(1):46–58. doi:10.1002/bit.20363.
- [10] Handel A, Longini Jr IM, Antia R. Towards a quantitative understanding of the within-host dynamics of influenza A infections. *J R Soc Interface.* 2010;7(42):35–47. doi:10.1098/rsif.2009.0067.
- [11] Lee HY, Topham DJ, Park SY, Hollenbaugh J, Treanor J, Mosmann TR, et al. Simulation and prediction of the adaptive immune response to influenza A virus infection. *J Virol.* 2009;83(14):7151–7165. doi:10.1128/JVI.00098-09.

- [12] Hancioglu B, Swigon D, Clermont G. A dynamical model of human immune response to influenza A virus infection. *J Theor Biol.* 2007;246(1):70–86. doi:10.1016/j.jtbi.2006.12.015.
- [13] Bocharov GA, Romanyukha AA. Mathematical model of antiviral immune response III. Influenza A virus infection. *J Theor Biol.* 1994;167(4):323–360.
