# Supplementary material for: Sequential infection experiments for quantifying innate and adaptive immunity during influenza infection
Source: arXiv:1709.02145 ancillary file (2018-06-05)
Supplement: Supplementary file 5 [file S2_Text.pdf]

# Sequential infection experiments for quantifying innate and adaptive immunity during influenza infection

## S2 Text:

Notes on biologically plausible ranges for the parameters  $p_{Vratio}$ ,  $\alpha$  and  $\gamma$

First, we examine the parameter  $\alpha$ . The concentration of virions in nasal wash is lower than the concentration of virions in the respiratory tract by a factor of  $a = 1 - 100$  [1]. The volume of the ferret upper respiratory tract, which was assumed to be the site of infection, is approximately  $v = 1\text{mL}$  [2], while the concentration of nasal wash was reported per  $b = 0.1\text{mL}$  [3]. We assumed that 1 RNA copy number corresponded to one (infectious or non-infectious) virion. Hence, the number of RNA copies/100 $\mu\text{L}$  of nasal wash corresponding to one virion in the respiratory tract ( $\alpha$ ) was  $(b/v)/a$ . Based on the bounds for  $a$  and  $b$ , the bounds for  $\alpha$  were then  $[10^{-3}, 10^{-1}]$ .

Next, we examine the parameter  $\gamma$ . Petrie *et al.* [4] used the bounds  $[10^0, 10^5]$  to fit the initial ratio of total to infectious virions. These bounds were in units of RNA copy number/TCID<sub>50</sub> ( $f$ ). These bounds were based on the variability across different inocula given to donor ferrets in the experiments by Butler *et al.* [5]; the study by Petrie *et al.* [4] analysed data from these experiments. However, in our study,  $\gamma$  was required to be in units of RNA copy number/virion, as we accounted for the loss of a single virion due to its infecting a target cell. Assays to measure the amount of infectious virus cannot measure the number of virions directly; hence, we needed to estimate the conversion factor between TCID<sub>50</sub> and virions ( $h$ ). At the minimum, one virion was required to establish an infection; hence, the lower bound for the number of virions corresponding to 1 TCID<sub>50</sub> was 1 virion. Handel *et al.* [1] estimated that 1 TCID<sub>50</sub> corresponds to 1–100 virions, so the bounds for  $h$  were  $[1, 100]$ . Hence, the initial ratio of total to infectious virions in the respiratory tract in units of RNA copy number/virion ( $\gamma$ ), which by definition had a lower bound of 1, was  $\gamma = f/h$ . Based on the bounds for  $f$  and  $h$ , the bounds for  $\gamma$  were then  $[10^0, 10^5]$ .

Lastly, we tackle the parameter  $p_{Vratio}$ . Petrie *et al.* [4] used the bounds  $[10^0, 10^6]$  to fit the ratio of production of total to infectious virions, in units of RNA copy number/TCID<sub>50</sub> ( $q$ ). These bounds were based on the variability of this ratio in the data provided by Butler *et al.* [5]. The ratio of production of total to infectious virions in units of RNA copy number/virion ( $p_{Vratio}$ ), which also by definition had a lower bound of 1, was then  $p_{Vratio} = q/h$ . Based on

the bounds for  $h$  and  $q$ , the bounds for  $p_{Vratio}$  were then  $[10^0, 10^6]$ .

## References

- [1] Handel A, Longini Jr IM, Antia R. Neuraminidase inhibitor resistance in influenza: assessing the danger of its generation and spread. PLoS Comput Biol. 2007;3(12):e240. doi:10.1371/journal.pcbi.0030240.
- [2] Petrie SM, Guarnaccia T, Laurie KL, Hurt AC, McVernon J, McCaw JM. Reducing uncertainty in within-host parameter estimates of influenza infection by measuring both infectious and total viral load. PLoS ONE. 2013;8(5):e64098. doi:10.1371/journal.pone.0064098.
- [3] Laurie KL, Guarnaccia TA, Carolan LA, Yan AWC, Aban M, Petrie S, et al. Interval between infections and viral hierarchy are determinants of viral interference following influenza virus infection in a ferret model. J Infect Dis. 2015;212(11):1701–1710. doi:10.1093/infdis/jiv260.
- [4] Petrie SM, Butler J, Barr IG, McVernon J, Hurt AC, McCaw JM. Quantifying relative within-host replication fitness in influenza virus competition experiments. J Theor Biol. 2015;382:259–271. doi:10.1016/j.jtbi.2015.07.003.
- [5] Butler J, Hooper KA, Petrie S, Lee R, Maurer-Stroh S, Reh L, et al. Estimating the fitness advantage conferred by permissive neuraminidase mutations in recent oseltamivir-resistant A(H1N1)pdm09 influenza viruses. PLoS Pathog. 2014;10(4):e1004065. doi:10.1371/journal.ppat.1004065.
