# Supplementary material for: Sequential infection experiments for quantifying innate and adaptive immunity during influenza infection
Source: arXiv:1709.02145 ancillary file (2018-06-05)
Supplement: Supplementary file 6 [file S2_table.pdf]

## S2 Table

| Parameter            | Description                                                                               | Value                           | Prior bounds               | Units             |
|----------------------|-------------------------------------------------------------------------------------------|---------------------------------|----------------------------|-------------------|
| $\log_{10} \delta_F$ | interferon decay rate                                                                     | $\log_{10} 2$                   | $[-1, 2]$ $[1, 2]$         | $\text{day}^{-1}$ |
| $\log_{10} \phi$     | (scaled) rate at which target cells become resistant to infection                         | $\log_{10}(3.3 \times 10^{-5})$ | $[-10, 0]$ $[3, 1]$        | $\text{day}^{-1}$ |
| $\log_{10} \rho$     | rate at which resistant cells become susceptible to infection                             | $\log_{10} 2$                   | $[0, 2]$ $[2, 4, 5, 6, 1]$ | $\text{day}^{-1}$ |
| $\log_{10} s$        | (scaled) factor by which the production rate of virions is decreased by type I interferon | $5 \times 10^{-4}$              | $[-10, 0]$                 | $\text{day}^{-1}$ |
| $\log_{10} \kappa_F$ | (scaled) clearance rate of infected cells by natural killer cells                         | $\log_{10}(2.5 \times 10^{-3})$ | $[-10, 0]$ $[1]$           | $\text{day}^{-1}$ |

1

## References

- [1] Pawelek KA, Huynh GT, Quinlivan M, Cullinane A, Rong L, Perelson AS. Modeling within-host dynamics of influenza virus infection including immune responses. *PLoS Comput Biol.* 2012;8(6):e1002588. doi:10.1371/journal.pcbi.1002588.
- [2] Bocharov GA, Romanyukha AA. Mathematical model of antiviral immune response III. Influenza A virus infection. *J Theor Biol.* 1994;167(4):323–360.
- [3] Saenz RA, Quinlivan M, Elton D, MacRae S, Blunden AS, Mumford JA, et al. Dynamics of influenza virus infection and pathology. *J Virol.* 2010;84(8):3974–3983. doi:10.1128/JVI.02078-09.
- [4] Hancioglu B, Swigon D, Clermont G. A dynamical model of human immune response to influenza A virus infection. *J Theor Biol.* 2007;246(1):70–86. doi:10.1016/j.jtbi.2006.12.015.
- [5] Heffernan JM, Keeling MJ. An in-host model of acute infection: measles as a case study. *Theor Popul Biol.* 2008;73(1):134–147. doi:10.1016/j.tpb.2007.10.003.
- [6] Chang DB, Young CS. Simple scaling laws for influenza A rise time, duration, and severity. *J Theor Biol.* 2007;246(4):621–635. doi:10.1016/j.jtbi.2007.02.004.
