# Supplementary material for: Sequential infection experiments for quantifying innate and adaptive immunity during influenza infection
Source: arXiv:1709.02145 ancillary file (2018-06-05)
Supplement: Supplementary file 9 [file S4_table.pdf]

## S4 Table

|   | Parameter            | Description                                                                                  | Value                      | Prior bounds          | Units                    |
|---|----------------------|----------------------------------------------------------------------------------------------|----------------------------|-----------------------|--------------------------|
|   | $\log_{10} k_B$      | concentration of viral RNA for half-maximal stimulation of naive B cells                     | $\log_{10}(2 \times 10^8)$ | [1, 10]               | RNA copy no./100 $\mu$ L |
|   | $\log_{10} \beta_B$  | maximal stimulation rate of naive B cells                                                    | $\log_{10} 1$              | [-5, 5]               | day <sup>-1</sup>        |
|   | $\log_{10} \tau_B$   | total proliferation time of plasmablasts                                                     | $\log_{10} 4$              | [0, 1] [1, 2]         | day                      |
|   | $\log_{10} \kappa_A$ | (scaled) neutralisation rate of virions by antibodies                                        | $\log_{10} 360$            | [-10, 10] [3]         | day <sup>-1</sup>        |
|   | $\log_{10} \delta_A$ | antibody decay rate                                                                          | $\log_{10} 0.04$           | [-2, -1] [4, 5]       | day <sup>-1</sup>        |
|   | $\log_{10} \delta_B$ | plasmablast and plasma cell decay rate                                                       | $\log_{10} 0.11$           | [-1, 0] [6, 7]        | day <sup>-1</sup>        |
|   | $\log_{10} \beta_C$  | maximal stimulation rate of naive/memory CD8 <sup>+</sup> T cells                            | $\log_{10} 1$              | [-5, 5]               | day <sup>-1</sup>        |
| † | $\log_{10} \tau_E$   | total proliferation time of effector CD8 <sup>+</sup> T cells                                | $\log_{10} 5$              | [0.5, 1] [8]          | day                      |
|   | $\log_{10} \delta_E$ | decay rate of effector CD8 <sup>+</sup> T cells                                              | $\log_{10} 0.6$            | [-1, 0] [9]           | day <sup>-1</sup>        |
|   | $\log_{10} \epsilon$ | proportion of effector CD8 <sup>+</sup> T cells which become memory CD8 <sup>+</sup> T cells | $\log_{10} 0.02$           | [-3, -1] [10, 11, 12] |                          |
|   | $\log_{10} \tau_M$   | mean refractory time for memory CD8 <sup>+</sup> T cells                                     | $\log_{10} 14$             | [1, 1.5] [13]         | day                      |
|   | $\sigma$             | measurement error                                                                            | 0.5                        | [0, 2]                |                          |

## References

- [1] Marchuk GI, Petrov RV, Romanyukha AA, Bocharov GA. Mathematical model of antiviral immune response. I. Data analysis, generalized picture construction and parameters evaluation for hepatitis B. *J Theor Biol.* 1991;151(1):1–40. doi:10.1016/S0022-5193(05)80142-0.
- [2] Sze DMY, Toellner KM, García de Vinuesa C, Taylor DR, MacLennan ICM. Intrinsic constraint on plasmablast growth and extrinsic limits of plasma cell survival. *J Exp Med.* 2000;192(6):813–821. doi:10.1084/jem.192.6.813.
- [3] Miao H, Hollenbaugh JA, Zand MS, Holden-Wiltse J, Mosmann TR, Perelson AS, et al. Quantifying the early immune response and adaptive immune response kinetics in mice infected with influenza A virus. *J Virol.* 2010;84(13):6687–6698. doi:10.1128/JVI.00266-10.
- [4] Bocharov GA, Romanyukha AA. Mathematical model of antiviral immune response III. Influenza A virus infection. *J Theor Biol.* 1994;167(4):323–360.
- [5] Lee HY, Topham DJ, Park SY, Hollenbaugh J, Treanor J, Mosmann TR, et al. Simulation and prediction of the adaptive immune response to influenza A virus infection. *J Virol.* 2009;83(14):7151–7165. doi:10.1128/JVI.00098-09.
- [6] Bortnick A, Allman D. What is and what should always have been: long-lived plasma cells induced by T cell-independent antigens. *J Immunol.* 2013;190(12):5913–5918. doi:10.4049/jimmunol.1300161.
- [7] Minges Wols HA. Plasma Cells. In: eLS. 2006. Chichester, UK: John Wiley & Sons, Ltd; 2015. p. 1–11.
- [8] Lehmann-Grube F, Assmann U, Löliger C, Moskopididis D, Löhler J. Mechanism of recovery from acute virus infection. I. Role of T lymphocytes in the clearance of lymphocytic choriomeningitis virus from spleens of mice. *J Immunol.* 1985;134(1):608–15.
- [9] Veiga-Fernandes H, Walter U, Bourgeois C, McLean A, Rocha B. Response of naïve and memory CD8+ T cells to antigen stimulation in vivo. *Nat Immunol.* 2000;1(1):47–53. doi:10.1038/76907.
- [10] Murali-Krishna K, Altman JD, Suresh M, Sourdive DJ, Zajac AJ, Miller JD, et al. Counting antigen-specific CD8 T cells: a reevaluation of bystander activation during viral infection. *Immunity.* 1998;8(2):177–87. doi:10.1016/S1074-7613(00)80470-7.
- [11] De Boer RJ, Oprea M, Antia R, Murali-Krishna K, Ahmed R, Perelson AS. Recruitment times, proliferation, and apoptosis rates during the CD8+ T-cell response to lymphocytic choriomeningitis virus. *J Virol.* 2001;75(22):10663–10669. doi:10.1128/JVI.75.22.10663-10669.2001.

- [12] Chao DL, Davenport MP, Forrest S, Perelson AS. A stochastic model of cytotoxic T cell responses. *J Theor Biol.* 2004;228(2):227–240. doi:10.1016/j.jtbi.2003.12.011.
- [13] Kaech SM, Hemby S, Kersh E, Ahmed R. Molecular and functional profiling of memory CD8 T cell differentiation. *Cell.* 2002;111(6):837–851. doi:10.1016/s0092-8674(02)01139-x.
